# Supplementary material for: Faster Optimization in S-Graphs Exploiting Hierarchy
Source: arXiv:2308.11242 source file (2023-08-22)
Supplement: Supplementary file 1 [file appendix.tex]

\section{Appendix}

This section provides all the tables used for computation of the percentage difference between \textit{S-Graphs+} and its relevant baselines. From Table~\ref{tab:percentage_simulated_data_s_graphs} it can be observed \textit{S-Graphs+} \mbox{w. OR} results in an improvement in accuracy of $5.44\%$ over \textit{S-Graphs}, \mbox{\textit{S-Graphs+} w. OF} shows a slight decrease in accuracy of $3.03\%$ over \textit{S-Graphs}, but overall  \textit{S-Graphs+} which combines the new room detector and newly proposed factors shows an improved accuracy of $13.37\%$ over its baseline. 

Table~\ref{tab:percentage_simulated_data_all} presents the percentage improvement of \textit{S-Graphs+} using VGICP odometry over all the baselines in the simulated dataset. \textit{S-Graphs+} shows improvement of $51.88\%$, $411.39\%$, $1298.6\%$, $500\%$, $2098.8\%$ over HDL-SLAM, ALOAM, MLOAM, FLOAM and LeGO-LOAM respectively.

\begin{table}[!htp]
\setlength{\tabcolsep}{4pt}
\scriptsize
\centering
\caption{Percentage increase in accuracy of \textit{S-Graphs+}, \mbox{\textit{S-Graphs+} w. OR} and \mbox{\textit{S-Graphs+} w. OF} with respect to \textit{S-Graphs} on simulated data. Best results are boldfaced.}
\begin{tabular}{l  l | c c c c c | c}
\toprule
\multicolumn{2}{l|}{\textbf{Method}} & \multicolumn{4}{l}{\textbf{Dataset} $\%$ $\boldsymbol{\uparrow}$}  \\
\midrule
{Mapping} & \multicolumn{1}{|l|} {Odometry} & \textit{C1F0} &  \textit{C1F2}  & \textit{SE1} & \textit{SE2} & \textit{SE3} & Avg \\
\midrule
{S-Graphs} \cite{s_graphs} \textit{(Baseline)} & \multicolumn{1}{|l|}{VGICP} & 0 & 0 & 0  & 0 & 0 & 0 \\  
\midrule
%{S-Graphs (NP)} & \multicolumn{1}{|l|}{VGICP} & 0.05 & {0.03} & 0.02 & \textbf{0.08} & 0.03 \\ 
%{S-Graphs (NF)} & \multicolumn{1}{|l|}{VGICP} & 0.05 & \textbf{0.02} & 0.02 & 0.09 & 0.04 \\
%{S-Graphs (NR)} & \multicolumn{1}{|l|}{VGICP} &   &  &  &  &  \\
\mbox{\textit{S-Graphs+} w. OR} & \multicolumn{1}{|l|}{VGICP} & 2.75 & 1.95 & 14.68  & \textbf{11.43} &  -3.63 & 5.44 \\
\mbox{\textit{S-Graphs+} w. OF} & \multicolumn{1}{|l|}{VGICP} & -4.32  & -16.73 & 0 &  7.69 &  -1.81 & -3.03 \\
%{S-Graphs (NF+NR)} & \multicolumn{1}{|l|}{VGICP} &   &  &  &  &  \\
%\textit{S-Graph+ w/o top layer} & \underline{4.20} & \underline{5.55} & & {48.4} & 5.14 & \textbf{31.17} & {15.22} & \textbf{17.19} & \textbf{15.22} & 21.46 & 27.70 \\ 
\midrule
\textit{S-Graphs+ (ours)} & \multicolumn{1}{|l|}{VGICP}  & \textbf{12.18} & \textbf{31.91} & \textbf{12.39} & -2.31  & \textbf{12.69} & \textbf{13.37} \\ 
\bottomrule
\end{tabular}
\label{tab:percentage_simulated_data_s_graphs}
\end{table}

\begin{table}[!htp]
\setlength{\tabcolsep}{3pt}
\scriptsize
\centering
\caption{Percentage decrease in accuracy of relevant baselines with respect to \textit{S-Graphs+} using VGICP odometry on simulated data. Best results are boldfaced.}
\begin{tabular}{l  l | c c c c c | c}
\toprule
\multicolumn{2}{l|}{\textbf{Method}} & \multicolumn{4}{l}{\textbf{Dataset} $\%$ $\boldsymbol{\downarrow}$}  \\
\midrule
{Mapping} & \multicolumn{1}{|l|} {Odometry} & \textit{C1F0} &  \textit{C1F2}  & \textit{SE1} & \textit{SE2} & \textit{SE3} & Avg \\
\midrule
HDL-SLAM \cite{hdl_graph_slam} & \multicolumn{1}{|l|} {VGICP \cite{vgicp}}  & 110.7 &  {21.14} & 28.80 & 13.86 & 84.87 & 51.87 \\ 
ALOAM \cite{loam} & \multicolumn{1}{|l|} {ALOAM} & 121.5 & 397.1 & 721.9 & 331.8 & 484.6 &  411.4 \\
MLOAM \cite{mloam} & \multicolumn{1}{|l|} {MLOAM} & - & 2768 & 3360 & -  & 364.8 & 1298 \\ 
FLOAM \cite{floam} & \multicolumn{1}{|l|} {FLOAM} & 161.7 & 728.5  & 664.4 & 227.6  & 718.9 & 500 \\ 
LeGO-LOAM \cite{lego-loam} & \multicolumn{1}{|l|} {LeGO-LOAM}  & - & - & - & - & 2099 & 2099 \\
{S-Graphs} \cite{s_graphs} & \multicolumn{1}{|l|}{VGICP} & 13.87 & 46.86 & 14.14  & -2.26 & {14.54} & 17.43 \\  \midrule
%{S-Graphs (NP)} & \multicolumn{1}{|l|}{VGICP} & 0.05 & {0.03} & 0.02 & \textbf{0.08} & 0.03 \\ 
%{S-Graphs (NF)} & \multicolumn{1}{|l|}{VGICP} & 0.05 & \textbf{0.02} & 0.02 & 0.09 & 0.04 \\
%{S-Graphs (NR)} & \multicolumn{1}{|l|}{VGICP} &   &  &  &  &  \\
\mbox{\textit{S-Graphs+} w. OR} & \multicolumn{1}{|l|}{VGICP} & {10.74} & 44.0 & \textbf{-2.62}  & \textbf{-13.43} &  18.69 & {11.48} \\
\mbox{\textit{S-Graphs+} w. OF} & \multicolumn{1}{|l|}{VGICP} & 18.79  & 71.43 & 14.14 &  -9.77 &  16.62 & 22.24 \\
%{S-Graphs (NF+NR)} & \multicolumn{1}{|l|}{VGICP} &   &  &  &  &  \\
%\textit{S-Graph+ w/o top layer} & \underline{4.20} & \underline{5.55} & & {48.4} & 5.14 & \textbf{31.17} & {15.22} & \textbf{17.19} & \textbf{15.22} & 21.46 & 27.70 \\ 
\midrule
\textit{S-Graphs+ (Baseline)} & \multicolumn{1}{|l|}{VGICP} & \textbf{0} & \textbf{0} & 0 & 0  & \textbf{0} & \textbf{0} \\ 
\textit{S-Graphs+} & \multicolumn{1}{|l|}{FLOAM} & 32.89 &  568.5  & 199.48 &  3.11 &  490.50 & 258.9 \\ 
\bottomrule
\end{tabular}
\label{tab:percentage_simulated_data_all}
\end{table}

\begin{table}[!htp]
\setlength{\tabcolsep}{4pt}
\caption{Percentage increase in accuracy \textit{S-Graphs+}, \mbox{\textit{S-Graphs+} w. OR} and \mbox{\textit{S-Graphs+} w. OF} with respect to \textit{S-Graphs} in real in-house dataset.}
\scriptsize
\centering
\begin{tabular}{l | c c c c c c c | c}
\toprule
& \multicolumn{3}{l}{\textbf{Dataset} (\%) $\boldsymbol{\uparrow}$} \\
\toprule
 {Mapping}  & \textit{C1F1} &  \textit{C1F2}  & \textit{C2F0} & \textit{C2F1} & \textit{C2F2} & \textit{C3F1} & \textit{C3F2} & Avg \\ 
\midrule
{S-Graphs} \cite{s_graphs} & 0 & 0 & 0 & 0 & 0  & 0 &  0 & 0 \\ 
\midrule
\mbox{\textit{S-Graphs+} w. OR}  & \textbf{2.11} & -0.53 & 3.80 & 8.72 & -3.41 & -5.7 & 14.16 &  2.74 \\ 
\mbox{\textit{S-Graphs+} w. OF} & 0.91 & -0.53 & 7.61 & 7.80 & \textbf{0} & -2.19 & 14.60 &  4.03 \\ 
\midrule
\textit{S-Graphs+ (Baseline)} & 0.60 & \textbf{0}  & \textbf{8.15} & \textbf{13.3} & \textbf{0} & \textbf{2.19} & \textbf{17.26} & \textbf{5.93}  \\ 
\bottomrule 
\end{tabular}
\label{tab:rmse_real_data_percentage_s_graphs}
\end{table}

\begin{table}[!htp]
\setlength{\tabcolsep}{3pt}
\caption{Percentage decrease in accuracy of relevant baselines with respect to \textit{S-Graphs+} on real in-house dataset. `-' refers to an unsuccessful run. Best results are boldfaced.}
\scriptsize
\centering
\begin{tabular}{l | c c c c c c c | c}
\toprule
& \multicolumn{3}{l}{\textbf{Dataset} (\%) $\boldsymbol{\downarrow}$} \\
\toprule
 {Mapping}  & \textit{C1F1} &  \textit{C1F2}  & \textit{C2F0} & \textit{C2F1} & \textit{C2F2} & \textit{C3F1} & \textit{C3F2} & Avg \\ 
\midrule
HDL-SLAM \cite{hdl_graph_slam} & 1.82 & 4.76  & 9.47 & 11.64 & 10.80 & 2.69 & 3.74 & 6.42 \\ 
ALOAM \cite{loam} & 59.88 & 77.78 & 101.8  & 138.6 & 69.89 & 63.68 & 132.1 & 91.96 \\ 
MLOAM \cite{mloam} & 36.78 &  46.03 & 140.2 & 71.43 & 34.09  & - & - &  46.94 \\ 
FLOAM \cite{floam}  & 108.2 & 107.4 & 137.7 & 193.7 & 124.43 & 161.4 & 107.5 & 134.4   \\
LeGO-LOAM \cite{lego-loam}  & - & - & 132.0 &  140.7 & - & 137.2 &  169.0 & 82.7 \\
{S-Graphs} \cite{s_graphs} & 0.61 & \textbf{0} & 8.88 & 15.34 & \textbf{0}  & {2.24} &  20.86 & 6.85 \\ 
%\textit{S-Graph - w/o top. layer} & {0.94} & \underline{0.333} & {1.42}   \\ 
\midrule
\mbox{\textit{S-Graphs+} w. OR}  & \textbf{-1.52} & {0.53} & 4.73 & {5.29} & 3.41 & 8.07 & 3.74 & 3.46 \\ 
\mbox{\textit{S-Graphs+} w. OF} & -0.3 & 0.53 & {0.59} & 6.35 & \textbf{0} & 4.48 & {3.21} & {2.12}  \\ 
\midrule
\textit{S-Graphs+ (Baseline)} & 0 & \textbf{0}  & \textbf{0} & \textbf{0} & \textbf{0}  & \textbf{0} & \textbf{0} & \textbf{0} \\ 
\bottomrule 
\end{tabular}
\label{tab:rmse_real_data_percentage_all}
\end{table}

Table~\ref{tab:rmse_real_data_percentage_s_graphs} shows the percentage improvement of \mbox{\textit{S-Graphs+} w. OR}, \mbox{\textit{S-Graphs+} w. OF} and \textit{S-Graphs+} over its baseline \textit{S-Graphs} in case of in-house real experiments. \mbox{\textit{S-Graphs+} w. OR} shows an improvement of $2.74\%$ over its baseline, while \mbox{\textit{S-Graphs+} w. OF} shows an improvement of $4.03\%$ with respect to its baseline. \textit{S-Graphs+} combining both the \mbox{\textit{S-Graphs+} w. OR} and \mbox{\textit{S-Graphs+} w. OF} shows an improved performance of $5.93\%$ over its baseline. 

Table~\ref{tab:rmse_real_data_percentage_all} shows the percentage improvement of \textit{S-Graphs+} over its baselines for in-house real experiments. \textit{S-Graphs+} offers improved performance by $6.42\%$, $91.96\%$, $46.94\%$, $134.36\%$, $82.70\%$ over the algorithms HDL-SLAM, ALOAM, MLOAM, FLOAM, and LeGO-LOAM respectively.   

\begin{table}[!htp]
\setlength{\tabcolsep}{4pt}
\centering
\caption{Percentage increase in accuracy of  \textit{S-Graphs+}, \mbox{\textit{S-Graphs+} w. OR} and \mbox{\textit{S-Graphs+} w. OF} with respect to the baseline \textit{S-Graphs} utilizing VGICP odometry. Best results are boldfaced.}
\scriptsize
\begin{tabular}{l l | c c c c c | c}
\toprule
\textbf{Method}  & & \multicolumn{4}{l}{\textbf{Dataset} (\%) $\boldsymbol{\uparrow}$} \\
\toprule
{Mapping} & \multicolumn{1}{|l|} {Odometry}  & \textit{T6} & 
\textit{T7}  & \textit{T8} & \textit{T10} & \textit{T11} & Avg \\ 
\midrule
{S-Graphs} \cite{s_graphs} \textit{(Baseline)} &  \multicolumn{1}{|l|}{VGICP} & 0 & 0 & 0 & 0 & 0 & 0 \\ 
\midrule
\mbox{\textit{S-Graphs+} w. OR} & \multicolumn{1}{|l|}{VGICP} & \textbf{1.17} & \textbf{1.49} & \textbf{6.55} & 48.87 & 8.73 & 13.36 \\
\mbox{\textit{S-Graphs+} w. OF} & \multicolumn{1}{|l|}{VGICP} & -3.52 & -1.12 & 6.27 & 44.29 & -4.31 & 8.32  \\
\midrule
\textit{S-Graphs+} & \multicolumn{1}{|l|}{VGICP} & 0 & 0.75 & 6.27 & \textbf{51.33} & \textbf{14.62} & \textbf{14.59} \\
\bottomrule
\end{tabular}
\label{tab:percentage_ate_tiers_dataset_s_graphs}
\end{table}

\begin{table}[!htp]
\setlength{\tabcolsep}{4pt}
\centering
\caption{Percentage decrease in accuracy of relevant baseline with respect to \textit{S-Graphs+} utilizing FLOAM odometry over the TIERS dataset \cite{tiers_dataset}. Best results are boldfaced.}
\scriptsize
\begin{tabular}{l l | c c c c c | c}
\toprule
\textbf{Method}  & & \multicolumn{4}{l}{\textbf{Dataset} (\%) $\boldsymbol{\downarrow}$} \\
\toprule
{Mapping} & \multicolumn{1}{|l|} {Odometry}  & \textit{T6} &  \textit{T7}  & \textit{T8} & \textit{T10} & \textit{T11} & Avg \\ 
\midrule
HDL-SLAM \cite{hdl_graph_slam} & \multicolumn{1}{|l|}{VGICP \cite{vgicp}} & 1.59 & 3.02 & \textbf{-3.43} & 208.3  & 373.8 & 116.6 \\ 
ALOAM \cite{loam} & \multicolumn{1}{|l|}{ALOAM} & 1.98 & 1.89 & 7.79 & {40.99} & 287.6 & 68.06 \\
MLOAM \cite{mloam} & \multicolumn{1}{|l|}{MLOAM} & 1.98  & \textbf{-1.51}  & 5.61 & 445.3 & \textbf{-21.78} & 85.93 \\ 
FLOAM \cite{floam} & \multicolumn{1}{|l|}{FLOAM} & 2.38 & -0.75 & 0.09 & 47.62 & 165.8 & 43.20 \\ 
% LIO-MAPPING \cite{lio_mapping} & 0.35 & 0.35 & 0.29 & 0.45 \\ 
LeGO-LOAM \cite{lego-loam} & \multicolumn{1}{|l|}{LeGO-LOAM} & 8.33 & 26.42 & 13.08 & 191.7 &  {12.54} & 50.42 \\
{S-Graphs} \cite{s_graphs} & \multicolumn{1}{|l|}{VGICP} &  1.59 & 1.13 & 9.35 & 438.5 & 213.7 & 132.9 \\ 
\midrule
\mbox{\textit{S-Graphs+} w. OR} & \multicolumn{1}{|l|}{VGICP} & {0.4} & {-0.38} & 2.18 & 175.3 & 186.3 & {72.77} \\
\mbox{\textit{S-Graphs+} w. OF} & \multicolumn{1}{|l|}{VGICP} & 5.16 & 2.26 & 2.49 & 200 & 227.2 & 87.42  \\
\midrule
 \textit{S-Graphs+} & \multicolumn{1}{|l|}{VGICP} & 1.59 & 0.38 & 2.49 & 162.1 & 167.8 & {66.87} \\
 \textit{S-Graphs+ (Baseline)} & \multicolumn{1}{|l|}{FLOAM} & \textbf{0} & 0 & 0 & \textbf{0} & 0 & \textbf{0} \\
\bottomrule
\end{tabular}
\label{tab:percentage_ate_tiers_dataset_all}
\end{table}

Table~\ref{tab:percentage_ate_tiers_dataset_s_graphs} shows the increase in the accuracy of \mbox{\textit{S-Graphs+} w. OR}, \mbox{\textit{S-Graphs+} w. OF} and \textit{S-Graphs+} over its baseline for tiers public dataset. \mbox{\textit{S-Graphs+} w. OR} show improved accuracy of $13.36\%$ and  \mbox{\textit{S-Graphs+} w. OF} shows an improved accuracy of $8.32\%$ over its baseline. While \textit{S-Graphs+} shows an improved accuracy of $14.59\%$ over its baseline.

Table~\ref{tab:percentage_ate_tiers_dataset_all} presents the percentage decrease of the accuracy of baselines over \textit{S-Graphs+} utilizing FLOAM odometry for the tiers public dataset. As can be seen from the table, HDL-SLAM, ALOAM, MLOAM, FLOAM, and LeGO-LOAM show an average decrease in accuracy of $116.64\%$, $68.06\%$, $85.93\%$, $43.20\%$ and $50.42\%$ respectively.
